# Supplementary material for: Efficient calculation of dispersion energy for multireference systems with Cholesky decomposition. Application to excited-state interactions
Source: arXiv:2306.01547 ancillary file (2023-06-02)
Supplement: Supplementary file 1 [file supp_info.pdf]

# Supporting Information: Efficient calculation of dispersion energy for multireference systems with Cholesky decomposition. Application to excited-state interactions.

Michał Hapka,[*,†] Agnieszka Krzemińska,[‡] Marcin Modrzejewski,[†] Michał Przybytek,[†] and Katarzyna Pernal[‡]

†*Faculty of Chemistry, University of Warsaw, ul. L. Pasteura 1, 02-093 Warsaw, Poland*

‡*Institute of Physics, Lodz University of Technology, ul. Wolczanska 217/221, 93-005 Lodz, Poland*

E-mail: michal.hapka@uw.edu.pl

## Contents

**1 Induction energy with multiconfigurational wave functions at the $m^4$ cost S-2**

**2 Additional Results S-4**

**References S-11**

# 1 Induction energy with multiconfigurational wave functions at the $m^4$ cost

Begin with the induction interaction energy expression introduced in ref S1

$$E_{\text{ind}}^{(2)} = E_{\text{ind}}^{(2)}(A \leftarrow B) + E_{\text{ind}}^{(2)}(B \leftarrow A) \quad , \tag{1}$$

$$E_{\text{ind}}^{(2)}(A \leftarrow B) = -4 \sum_{\mu \in A} \frac{\left( \sum_{p>q \in A} \left[ \tilde{\mathbf{Y}}_{\mu}^{A} \right]_{pq} \bar{\Omega}_{pq}^{B} \right)^2}{\omega_{\mu}^{A}} \quad , \tag{2}$$

[$E_{\text{ind}}^{(2)}(B \leftarrow A)$ is defined analogously to $E_{\text{ind}}^{(2)}(A \leftarrow B)$], where $\bar{\Omega}^B$ is a vector of the modified interaction potential defined as

$$\forall_{p>q \in A} \quad \bar{\Omega}_{pq}^{B} = \left( n_p^{1/2} + n_q^{1/2} \right) \langle p | \hat{\Omega}_B | q \rangle \tag{3}$$

$$\hat{\Omega}_B(\mathbf{r}) = v^B(\mathbf{r}) + \int \frac{\rho^B(\mathbf{r}')}{|\mathbf{r} - \mathbf{r}'|} \mathrm{d}\mathbf{r}' \quad . \tag{4}$$

Equations are written in the natural orbitals representation of the monomer A and $n_p, n_q$ denote natural occupation numbers, $\forall_p \ 0 \leq n_p \leq 1$. Using the expression for the frequency-dependent density response function [see Eq. (6) in the main text]

$$\left[ \mathbf{C}^A(\omega) \right]_{pq,p'q'} = 2 \sum_{\nu} \left[ \tilde{\mathbf{Y}}_{\nu}^{A} \right]_{pq} \left[ \tilde{\mathbf{Y}}_{\nu}^{A} \right]_{p'q'} \frac{\omega_{\nu}^{A}}{\omega^2 + (\omega_{\nu}^{A})^2} \quad , \tag{5}$$

taken at $\omega = 0$ leads to

$$E_{\text{ind}}^{(2)}(A \leftarrow B) = -2 \left[ \bar{\mathbf{C}}^A(0) \right]^{\mathrm{T}} \bar{\Omega}^B \quad , \tag{6}$$

where

$$\forall_{p>q \in A} \quad \left[ \bar{\mathbf{C}}^A(0) \right]_{pq} = \sum_{p'>q' \in A} [\mathbf{C}^A(0)]_{pq,p'q'} \bar{\Omega}_{p'q'}^{B} \tag{7}$$

(analogous equations hold for the monomer $B$). The vector $\bar{\mathbf{C}}^A(0)$ can be easily found from Eq. (8) in the main text, written for $\omega = 0$ and projected on $\bar{\Omega}^B$,

$$\mathcal{A}_+\mathcal{A}_-\bar{\mathbf{C}}^A(0) = \mathcal{A}_+\bar{\Omega}^B \tag{8}$$

where the $\mathcal{A}_+$, $\mathcal{A}_-$ are the hessian matrices constructed for the monomer $A$. Multiply Eq. (8) by $[\mathcal{A}_+]^{-1}$ to obtain

$$\mathcal{A}_-\bar{\mathbf{C}}^A(0) = \bar{\Omega}^B \quad . \tag{9}$$

Splitting $\mathcal{A}_-$ into zeroth- and first-order terms in the coupling constant $\alpha$, see Eq. (13) in the main text taken for $\alpha = 1$,

$$\mathcal{A}_- = \mathcal{A}_-^{(0)} + \mathcal{A}_-^{(1)} \tag{10}$$

leads to

$$\bar{\mathbf{C}}^A(0) = [\mathcal{A}_-^{(0)}]^{-1}\bar{\Omega}^B - [\mathcal{A}_-^{(0)}]^{-1}\mathcal{A}_-^{(1)}\bar{\mathbf{C}}^A(0) \quad , \tag{11}$$

which gives rise to the iterative scheme

$$[\bar{\mathbf{C}}^A(0)]_{i+1} = [\bar{\mathbf{C}}^A(0)]_0 - [\mathcal{A}_-^{(0)}]^{-1}\mathcal{A}_-^{(1)}[\bar{\mathbf{C}}^A(0)]_i \quad , \tag{12}$$

where

$$[\bar{\mathbf{C}}^A(0)]_0 = [\mathcal{A}_-^{(0)}]^{-1}\bar{\Omega}^B \quad . \tag{13}$$

As it has been discussed in the main text, the matrix $\mathcal{A}_-^{(0)}$ is block diagonal with the largest blocks of the $M_{s_2}^2 \times M_{s_2}^2$ size, where $M_{s_2}$ denotes the number of the active orbitals. Consequently, the cost of its inversion is negligible if the number of the active orbitals is much smaller than that of the virtual orbitals. All matrix multiplications in the proposed iterative are of the $m^4$ cost.

The iterative algorithm presented in Eq. (12), has been implemented in GammCor using the DIIS accelaration technique.

## 2 Additional Results

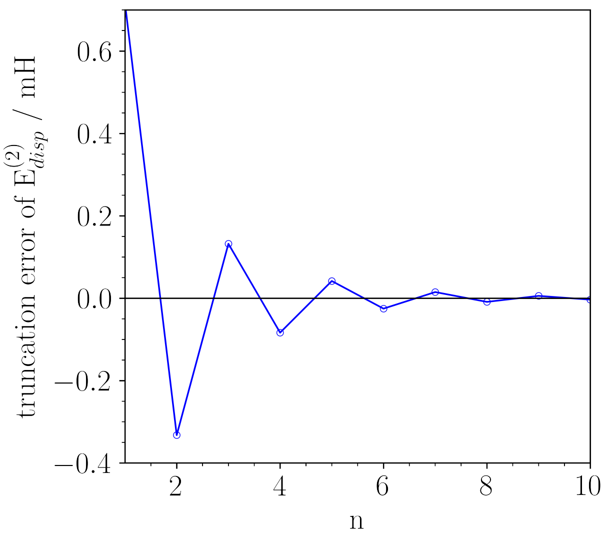


Figure S1: Convergence of the $E^{(2)}_{\mathrm{disp}}$ energy component as a function of the $n$-parameter, see Eqs.(11) and (14) in the main text, computed for benzen-cyclopentane complex in ground-state. Results obtained for aug-cc-pVTZ basis set.

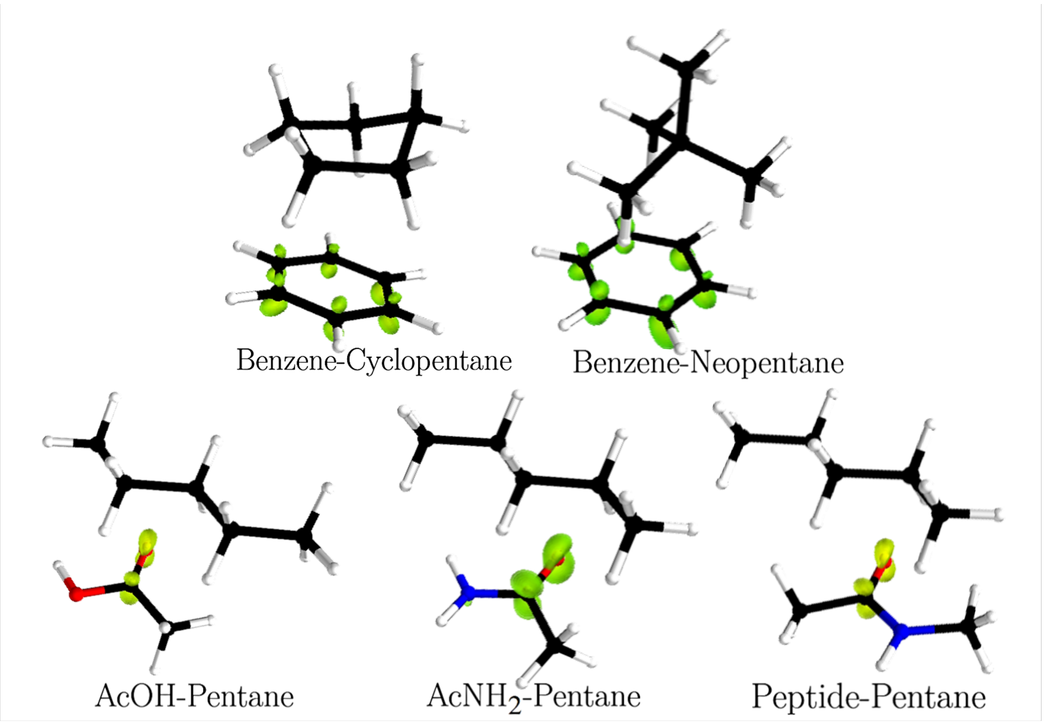


Figure S2: Differences of density between ground and $\pi \rightarrow \pi^*$ and $n \rightarrow \pi^*$ excited states respectively. Each isosurface consists of 6 contours of the difference density, generated to encompass 50%, 40%, 30%, 20%, 10% and 1% of the overall density, respectively.

Table S1: Convergence of the dispersion energy with $n = 6, 8, \ldots, 14$ with respect to the SAPT(CAS) reference. $E_{\rm disp}^{(2)}$ is the reference SAPT(CAS) dispersion energy. Basis set is aug-cc-pVTZ. Energy unit is $\mu E_h$.

| ground state | 6 | 8 | 10 | 12 | 14 | $E_{\rm disp}^{(2)}$ |
|---|---|---|---|---|---|---|
| benzene-$H_2O$ | −10.9 | −4.0 | −1.6 | −0.6 | −0.2 | −4859 |
| benzene-MeOH | −16.1 | −6.0 | −2.4 | −1.0 | −0.4 | −7763 |
| benzene-$MeNH_2$ | −14.5 | −5.2 | −2.0 | −0.8 | −0.3 | −7713 |
| pyridine-$H_2O$ | −29.7 | −15.1 | −8.0 | −4.4 | −2.4 | −6499 |
| pyridine-MeOH | −36.5 | −18.6 | −9.9 | −5.4 | −3.0 | −7948 |
| pyridine-$MeNH_2$ | −26.3 | −11.9 | −5.9 | −3.1 | −1.7 | −8217 |
| peptide-$H_2O$ | −8.3 | −3.1 | −1.2 | −0.5 | −0.2 | −4652 |
| peptide-$MeNH_2$ | −9.4 | −2.9 | −0.9 | −0.3 | −0.1 | −9057 |
| MAE | 19.0 | 8.4 | 4.0 | 2.0 | 1.0 | |
| MAX | 36.5 | 18.6 | 9.9 | 5.4 | 3.0 | |
| | | | | | | |
| excited state | 6 | 8 | 10 | 12 | 14 | ref. |
| benzene-$H_2O$ | −6.7 | −2.1 | −0.7 | −0.3 | −0.1 | −4589 |
| benzene-MeOH | −9.4 | −2.9 | −1.0 | −0.4 | −0.1 | −7377 |
| benzene-$MeNH_2$ | −8.0 | −2.1 | −0.6 | −0.2 | −0.1 | −7367 |
| pyridine-$H_2O$ | −15.4 | −5.8 | −2.1 | −0.6 | −0.1 | −6459 |
| pyridine-MeOH | −18.9 | −7.2 | −2.6 | −0.8 | −0.2 | −7891 |
| pyridine-$MeNH_2$ | −14.0 | −4.3 | −1.2 | −0.2 | 0.1 | −7978 |
| peptide-$H_2O$ | −8.0 | −3.0 | −1.2 | −0.5 | −0.2 | −4674 |
| peptide-$MeNH_2$ | −9.2 | −2.7 | −0.7 | −0.2 | 0.0 | −9217 |
| MAE | 11.2 | 3.8 | 1.3 | 0.4 | 0.1 | |
| MAX | 18.9 | 7.2 | 2.6 | 0.8 | 0.2 | |

Table S2: **Ground-state** interaction energies (in kcal/mol) at the SAPT(DFT) and SAPT(CAS) levels of theory. "ref." denotes supermolecular CCSD(T)/CBS results of Ref. S2; aV$XZ$ stands for aug-cc-pV$XZ$ ($X$=D,T,Q) basis sets of Dunning. The SAPT/CBS values were obtained using a two-point aVTZ→aVTZ extrapolation scheme of Halkier et al.[S3] SAPT(DFT) calculations were performed with localized PBE0AC xc potentials for the monomers[S4] and the ALDA xc kernel. All SAPT values include the $\delta_{\rm HF}$ correction.

| | SAPT(DFT) | | | SAPT(CAS) | | ref |
|---|---|---|---|---|---|---|
| | aVTZ | aVQZ | CBS | aVDZ | aVTZ | |
| benzen-cyclopentane | −3.35 | −3.45 | −3.52 | −3.25 | −3.63 | −3.51 |
| benzen-neopentane | −2.71 | −2.78 | −2.83 | −2.66 | −2.95 | −2.85 |
| AcOH-pentane | −2.61 | −2.70 | −2.77 | −2.46 | −2.82 | −2.91 |
| $AcNH_2$-pentane | −3.25 | −3.36 | −3.44 | −3.15 | −3.61 | −3.53 |
| peptide-pentane | −3.86 | −3.98 | −4.07 | −3.79 | −4.26 | −4.26 |

Table S3: **Ground-state** interaction energy components (in milliHartree) at the **SAPT(DFT)** level of theory. aV$X$Z stands for aug-cc-pV$X$Z ($X$=T,Q) basis sets of Dunning. SAPT(DFT) calculations were performed with localized PBE0AC xc potentials for the monomers[S4] and the ALDA xc kernel. Second-order exchange energy terms given in the $S^2$ approximation.

| | $X$ | $E^{(1)}_{\text{elst}}$ | $E^{(1)}_{\text{exch}}$ | $E^{(2)}_{\text{ind}}$ | $E^{(2)}_{\text{exch-ind}}$ | $E^{(2)}_{\text{disp}}$ | $E^{(2)}_{\text{exch-disp}}$ | $\delta_{\text{HF}}$ | $E^{\text{SAPT}+\delta_{\text{HF}}}_{\text{int}}$ |
|---|---|---|---|---|---|---|---|---|---|
| Benzene- | T | −3.713 | 9.995 | −3.192 | 2.958 | −12.331 | 1.697 | −0.760 | −5.346 |
| -Cyclopentane | Q | −3.709 | 9.986 | −3.193 | 2.959 | −12.539 | 1.752 | −0.760 | −5.503 |
| Benzene- | T | −3.018 | 7.929 | −2.479 | 2.238 | −9.769 | 1.333 | −0.560 | −4.326 |
| Neopentane | Q | −3.014 | 7.925 | −2.478 | 2.238 | −9.922 | 1.374 | −0.551 | −4.428 |
| AcOH- | T | −2.984 | 8.304 | −2.446 | 2.029 | −9.738 | 1.121 | −0.439 | −4.152 |
| -pentane | Q | −2.981 | 8.299 | −2.448 | 2.031 | −9.928 | 1.167 | −0.442 | −4.302 |
| $AcNH_2$- | T | −3.993 | 10.293 | −3.419 | 2.507 | −11.407 | 1.463 | −0.628 | −5.183 |
| -pentane | Q | −3.989 | 10.288 | −3.422 | 2.509 | −11.636 | 1.522 | −0.631 | −5.359 |
| peptide- | T | −4.424 | 11.958 | −3.583 | 2.808 | −13.959 | 1.728 | −0.678 | −6.147 |
| -pentane | Q | −4.417 | 11.947 | −3.583 | 2.807 | −14.219 | 1.794 | −0.679 | −6.350 |

Table S4: **Ground-state** interaction energy components (in milliHartree) at the **SAPT(CAS)** level of theory. aV$X$Z stands for aug-cc-pV$X$Z ($X$=D,T) basis sets of Dunning. All exchange energy terms given in the $S^2$ approximation. $E^{(2)}_{\text{exch-ind}}$ and $E^{(2)}_{\text{exch-ind}}$ in aVTZ are obtained via scaling, see Computational Details.

| | $X$ | $E^{(1)}_{\text{elst}}$ | $E^{(1)}_{\text{exch}}$ | $E^{(2)}_{\text{ind}}$ | $E^{(2)}_{\text{exch-ind}}$ | $E^{(2)}_{\text{disp}}$ | $E^{(2)}_{\text{exch-disp}}$ | $\delta_{\text{HF}}$ | $E^{\text{SAPT}+\delta_{\text{HF}}}_{\text{int}}$ |
|---|---|---|---|---|---|---|---|---|---|
| Benzene- | D | −3.329 | 8.549 | −2.220 | 1.961 | −10.686 | 1.305 | −0.751 | −4.419 |
| -cyclopentane | T | −3.270 | 8.496 | −2.305 | 2.036 | −11.362 | 1.388 | −0.760 | −5.777 |
| Benzene- | D | −2.546 | 6.536 | −1.494 | 1.241 | −8.397 | 0.985 | −0.551 | −3.675 |
| -neopentane | T | −2.523 | 6.503 | −1.599 | 1.327 | −8.896 | 1.044 | −0.560 | −4.703 |
| AcOH- | D | −2.426 | 6.614 | −1.567 | 1.239 | −8.071 | 0.769 | −0.439 | −3.442 |
| -pentane | T | −2.451 | 6.693 | −1.680 | 1.328 | −8.843 | 0.843 | −0.440 | −4.549 |
| AcNH2- | D | −3.371 | 8.389 | −2.392 | 1.536 | −9.606 | 1.052 | −0.620 | −4.391 |
| -pentane | T | −3.337 | 8.351 | −2.495 | 1.603 | −10.379 | 1.197 | −0.628 | −5.689 |
| peptide- | D | −3.708 | 9.723 | −2.393 | 1.756 | −11.905 | 1.262 | −0.673 | −5.265 |
| -pentane | T | −3.682 | 9.674 | −2.503 | 1.836 | −12.798 | 1.357 | −0.678 | −6.793 |

Table S5: **Excited-state** interaction energy components (in milliHartree) at the **SAPT(CAS)** level of theory. aV$X$Z stands for aug-cc-pV$X$Z ($X$=D,T) basis sets of Dunning. All exchange energy terms given in the $S^2$ approximation. $E^{(2)}_{\text{exch-ind}}$ and $E^{(2)}_{\text{exch-ind}}$ in aVTZ are obtained via scaling, see Computational Details.

| | $X$ | $E^{(1)}_{\text{elst}}$ | $E^{(1)}_{\text{exch}}$ | $E^{(2)}_{\text{ind}}$ | $E^{(2)}_{\text{exch-ind}}$ | $E^{(2)}_{\text{disp}}$ | $E^{(2)}_{\text{exch-disp}}$ | $\delta_{\text{CAS}}$ | $E^{\text{SAPT}+\delta_{\text{CAS}}}_{\text{int}}$ |
|---|---|---|---|---|---|---|---|---|---|
| Benzene- | D | −3.115 | 8.259 | −2.183 | 2.007 | −10.329 | 1.226 | −0.739 | −4.873 |
| -cyclopentane | T | −3.054 | 8.209 | −2.260 | 2.078 | −10.987 | 1.305 | −0.746 | −5.455 |
| Benzene- | D | −2.306 | 6.202 | −1.456 | 1.269 | −8.088 | 0.910 | −0.537 | −4.005 |
| -neopentane | T | −2.280 | 6.172 | −1.551 | 1.352 | −8.570 | 0.964 | −0.543 | −4.456 |
| AcOH- | D | −2.493 | 6.624 | −1.596 | 1.410 | −8.300 | 0.825 | −0.447 | −3.977 |
| -pentane | T | −2.433 | 6.562 | −1.648 | 1.456 | −8.940 | 0.889 | −0.432 | −4.546 |
| AcNH2- | D | −3.538 | 9.141 | −3.115 | 3.051 | −9.858 | 1.202 | −0.808 | −3.924 |
| -pentane | T | −3.484 | 9.074 | −3.265 | 3.198 | −10.614 | 1.294 | −0.822 | −4.619 |
| peptide- | D | −3.669 | 9.827 | −2.374 | 2.107 | −12.042 | 1.306 | −0.667 | −5.512 |
| -pentane | T | −3.611 | 9.741 | −2.448 | 2.173 | −12.915 | 1.400 | −0.663 | −6.322 |

Table S6: Total CASSCF energies (in Hartree) computed for the dimer and monomers in their ground and excited states in aug-cc-pVTZ.

| | dimer | monomerA | monomerB |
|---|---|---|---|
| | | ground state | |
| Benzene-Cyclopentan | −426.078 533 | −230.852 756 | −195.230 155 |
| Benzene-Neopentane | −427.254 009 | −196.404 550 | −230.852 749 |
| AcOH-Pentane | −424.433 227 | −228.032 321 | −196.404 380 |
| AcNH2-Pentane | −404.530 470 | −208.129 818 | −196.404 349 |
| Peptide-Pentane | −443.606 199 | −196.404 355 | −247.206 538 |
| | | excited state | |
| Benzene-Cyclopentan | −425.894 636 | −230.668 890 | −195.230 155 |
| Benzene-Neopentane | −427.254 009 | −196.404 550 | −230.852 749 |
| AcOH-Pentane | −424.175 736 | −227.774 967 | −196.404 380 |
| AcNH2-Pentane | −404.308 504 | −207.909 109 | −196.404 349 |
| Peptide-Pentane | −443.365 463 | −246.966 172 | −196.404 355 |

Table S7: Errors of the dispersion energy with $n = 4, 6, \ldots, 20$ with respect to the SAPT(CAS) reference for the **A24 dataset**. "ref." denotes SAPT(CAS) values. MAE and MAX are mean absolute error and maximum error, respectively. Basis set is aug-cc-pVTZ. Energy unit is $\mu E_h$.

| | 4 | 6 | 8 | 10 | 12 | 20 | ref |
|---|---|---|---|---|---|---|---|
| $H_2O\cdots H_2O$ | 1.6 | −0.2 | 0.2 | 0.5 | 0.6 | 0.7 | −4428 |
| $H_2O\cdots NH_3$ | 2.2 | 0.2 | 0.6 | 0.8 | 0.9 | 1.0 | −6229 |
| $HCN\cdots HCN$ | 15.4 | 7.3 | 4.5 | 2.8 | 1.7 | 0.3 | −2918 |
| $HF\cdots HF$ | 4.8 | 0.1 | −0.3 | −0.2 | −0.1 | −0.1 | −3142 |
| $NH_3\cdots NH_3$ | 1.6 | 0.7 | 0.8 | 0.9 | 1.0 | 1.0 | −3899 |
| $C_2H_2\cdots C_2H_2$ | 0.8 | 1.4 | 1.0 | 0.7 | 0.5 | 0.3 | −2295 |
| $C_2H_4\cdots C_2H_4$ | −6.8 | −2.3 | −0.9 | −0.4 | −0.1 | 0.0 | −3471 |
| $CH_4\cdots C_2H_4$ | 1.7 | 0.8 | 0.5 | 0.4 | 0.3 | 0.3 | −1506 |
| $H_2O\cdots C_2H_4$ | 0.2 | −0.6 | −0.2 | 0.1 | 0.2 | 0.3 | −3734 |
| $H_2O\cdots CH_4$ | 3.4 | 1.0 | 0.5 | 0.4 | 0.3 | 0.3 | −1441 |
| $HCOH\cdots C_2H_4$ | 1.7 | 3.4 | 3.7 | 3.5 | 3.1 | 1.7 | −3570 |
| $HCOH\cdots HCOH$ | 21.7 | 16.9 | 13.7 | 11.1 | 8.9 | 4.1 | −7266 |
| $HF\cdots CH_4$ | 6.0 | 1.3 | 0.3 | 0.0 | 0.0 | −0.1 | −2461 |
| $NH_3\cdots C_2H_4$ | −1.4 | −0.7 | −0.1 | 0.1 | 0.2 | 0.3 | −2699 |
| $NH_3\cdots CH_4$ | 3.3 | 1.3 | 0.7 | 0.4 | 0.4 | 0.3 | −1821 |
| $Ar\cdots C_2H_4$ | 0.1 | −0.1 | 0.2 | 0.4 | 0.4 | 0.5 | −1195 |
| $BH_3\cdots CH_4$ | 73.7 | 62.6 | 54.1 | 47.1 | 41.3 | 25.5 | −4636 |
| $C_2H_2\cdots C_2H_2$ | −0.1 | 0.7 | 0.4 | 0.2 | 0.1 | 0.0 | −3348 |
| $C_2H_4\cdots C_2H_2$ | −6.2 | −1.8 | −0.7 | −0.3 | −0.1 | 0.0 | −3893 |
| $C_2H_4\cdots C_2H_4$ | −14.6 | −5.4 | −2.3 | −1.0 | −0.4 | 0.0 | −4507 |
| $CH_4\cdots C_2H_6$-1 | 5.1 | 1.9 | 1.4 | 0.8 | 0.5 | 0.3 | −2727 |
| $CH_4\cdots C_2H_6$-2 | 3.3 | 1.4 | 0.5 | 0.1 | −0.1 | −0.2 | −1995 |
| $CH_4\cdots CH_4$ | 2.8 | 1.0 | 0.3 | −0.1 | −0.2 | −0.3 | −1771 |
| MAE | 7.8 | 4.9 | 4.0 | 3.1 | 2.8 | 1.6 | |
| MAX | 73.7 | 62.6 | 54.1 | 47.1 | 41.3 | 25.5 | |

Table S8: Convergence of the dispersion energy with $n = 4, 6, \ldots, 20$ with respect to the SAPT(CAS) reference for the **TK21 dataset**. "ref." denotes SAPT(CAS) values. Basis set is aug-cc-pVTZ. Energy unit is $\mu E_h$.

| | 6 | 8 | 10 | 12 | 14 | ref |
|---|---|---|---|---|---|---|
| $F^- \cdots HF$ | −17.2 | −12.5 | −6.6 | −3.3 | −1.7 | −22 754 |
| $F^- \cdots H_2O$ | −8.6 | −6.8 | −3.6 | −1.7 | −0.7 | −14 237 |
| $Na^+ \cdots H_2O$ | −0.2 | −0.1 | 0.0 | 0.0 | 0.0 | −858 |
| $HF \cdots HF$ | 0.2 | −0.2 | −0.1 | 0.0 | 0.0 | −2959 |
| $CH_4 \cdots CH_4$ | 1.0 | 0.3 | 0.0 | −0.1 | −0.2 | −1525 |
| $H_2O \cdots H_2O$ | −0.9 | −0.5 | −0.2 | −0.1 | 0.0 | −4700 |
| $NH_3 \cdots CH_4$ | 0.7 | 0.3 | 0.1 | 0.0 | 0.0 | −1882 |
| $NH_3 \cdots H_2O$ | −0.8 | −0.4 | −0.2 | −0.1 | 0.0 | −6402 |
| $N_2 \cdots N_2$ | 0.1 | 0.0 | 0.0 | 0.0 | 0.0 | −728 |
| $C_2H_2 \cdots C_2H_2$(PD) | 1.4 | 1.0 | 0.6 | 0.4 | 0.3 | −2278 |
| $C_2H_2 \cdots C_2H_2$(S) | 0.2 | 0.2 | 0.1 | 0.1 | 0.1 | −1084 |
| $C_2H_2 \cdots C_2H_2$(T) | 1.2 | 0.8 | 0.6 | 0.4 | 0.3 | −2219 |
| $C_2H_6 \cdots HCN$ | 0.7 | 0.4 | 0.3 | 0.1 | 0.1 | −1809 |
| NCCN⋯NCCN | −20.8 | −14.1 | −10.1 | −7.4 | −5.5 | −3202 |
| $P_2 \cdots P_2$ | 0.5 | 0.3 | 0.2 | 0.1 | 0.1 | −3264 |
| $N_2O \cdots He$(GM) | 1.8 | 0.4 | 0.1 | 0.0 | 0.0 | −508 |
| $N_2O \cdots He$(LM) | 1.0 | 0.2 | 0.1 | 0.0 | 0.0 | −261 |
| $CO_2 \cdots He$(GM) | 1.6 | 0.4 | 0.1 | 0.0 | 0.0 | −457 |
| $CO_2 \cdots He$(LM) | 0.8 | 0.2 | 0.1 | 0.0 | 0.0 | −204 |
| Ar⋯Ar | −0.4 | −0.1 | 0.0 | 0.0 | 0.0 | −519 |
| PCCP⋯PCCP | 1.7 | 2.8 | 1.9 | 1.2 | 0.7 | −7913 |
| | | | | | | |
| MAE | 3.0 | 2.0 | 1.2 | 0.7 | 0.5 | |
| MAX | 20.8 | 14.1 | 10.1 | 7.4 | 5.5 | |

# References


(S1) Hapka, M.; Przybytek, M.; Pernal, K. Symmetry-Adapted Perturbation Theory Based on Multiconfigurational Wave Function Description of Monomers. *J. Chem. Theory Comput.* **2021**, *17*, 5538–5555.

(S2) Řezáč, J.; Riley, K. E.; Hobza, P. S66: A Well-balanced Database of Benchmark Interaction Energies Relevant to Biomolecular Structures. *J. Chem. Theory Comput.* **2011**, *7*, 2427–2438.

(S3) Halkier, A.; Helgaker, T.; Jørgensen, P.; Klopper, W.; Koch, H.; Olsen, J.; Wilson, A. K. Basis-set convergence in correlated calculations on Ne, $N_2$, and $H_2O$. *Chem. Phys. Lett.* **1998**, *286*, 243–252.

(S4) Heßelmann, A.; Jansen, G.; Schütz, M. Density-functional theory-symmetry-adapted intermolecular perturbation theory with density fitting: A new efficient method to study intermolecular interaction energies. *J. Chem. Phys.* **2005**, *122*, 014103.
